# Supplementary material for: FairRelay: Fair and Cost-Efficient Peer-to-Peer Content Delivery through Payment Channel Networks
Source: arXiv:2405.02973 source file (2024-05-05)
Supplement: Supplementary file 1 [file appendix.tex]

\textbf{On-chain Arbiter Smart Contract}
The on-chain arbiter contract follow a simple idea: if a delivery path $p_k$ is challenged by $\mathcal{P}$, in path $p_k$, all relays from right to left should reveal their mask secret in order. The maxium delay for each relay to reveal its mask secret is $\Delta_3$. If a relay fails to reveal its mask secret in time, it will be punished and $\mathcal{P}$ will get a compensation. The contract will also check if the challenge request is valid, and if the challenge request is valid, the contract will unlock the payment for $\mathcal{P}$.
\begin{algorithm}
    \caption{Payment Enfocement Contract}
    \begin{algorithmic}[3] % The [1] ensures lines are numbered
        \STATE \textbf{Maintain:} $\Delta_3$, $STATE$, $N$,$s$, $Logs: [hash] \rightarrow lists$
        \STATE \textbf{Procedure} Challenge($UC$, $\sigma_{UC}$, $\{\sigma_{UC_{k,i}}\}$, $s'$)

%%$UC : = (T_2, \mathbb{H}_{k,1},H(s_{sync}), ADDR_k )$
        \STATE \textbf{require: $UC.H(s_{sync}) == H(s')$}
        \STATE \textbf{require: $UC.T_2 > \text{current\_time}$}
        \STATE \textbf{require: UC is signed by all nodes in $UC.ADDR_k$}
        \STATE $s:= s'$

        \STATE $Logs[\text{H}(UC)] \leftarrow []$

        \STATE Set $Logs[\text{H}(UC)].state$ to "ACTIVATE"
        \STATE $N = |UC.ADDR_k|$

        \STATE \textbf{Procedure} Log($H{UC}$, $i$, $payload$)
        \IF{$H{UC}$ in $Logs$ AND $Logs[H{UC}].state == \text{"ACTIVATE"}$}
            \IF{H(payload) == $UC.H[i]$}
            \STATE $Logs[H{UC}].push((payload, current\_time)$
            \ENDIF 
        \ENDIF
        
        \STATE \textbf{Procedure} Punish($H{UC}$,  $i$)
        \STATE \textbf{require:} Punish call is issued by the first address of  $UC.ADDR_k$.
        \IF{ $Logs[H{UC}].state == \text{"ACTIVATE"}$}
        
            \STATE $log_p = Logs[H{UC}][i-1]$
            \STATE $log_n = Logs[H{UC}][i]$
            \STATE \textbf{require:} $log_p \neq nil $
            \IF{$log_n[1] - log_p[1] > \Delta_3$ or $log_n == nil$}
                \STATE Slash $UC'[i].Pk$'s deposit and compensate $\mathcal{P}$
                \STATE Set $Logs[H{UC}].state$ to "PUNISHED"
            \ENDIF
        \ENDIF

    \end{algorithmic}
\end{algorithm}
